# Supplementary material for: A Game-Theoretic Framework for Controlled Islanding in the Presence of Adversaries
Source: arXiv:2108.01628 source file (2021-09-27)
Supplement: Supplementary file 1 [file appendix.tex]

\section*{Appendix}

\subsection*{Sets}
\begin{tabular}{lll}
   $\mathcal{N}$  && The set of generators\\
   $\mathcal{D}$ && The set of load demands\\
   $\mathcal{B}$   && The set of substations\\
   $\mathcal{L}$ && The set of transmission lines\\
   $\mathcal{B}_k$ && The subset of substations $\mathcal{B}_k\subset\mathcal{B}$ corresponding to subsystem $\mathcal{G}_k$\\
   $\mathcal{L}_k$ && The subset of transmission lines $\mathcal{L}_k\subset\mathcal{L}$ corresponding to subsystem $\mathcal{G}_k$\\
\end{tabular}

\subsection*{Parameters}
\begin{tabular}{lll}
   $C$  &    & The substation compromise budget of the adversary\\
   $Z$ && A sufficiently large positive constant\\
   $P_{i,j}$ && The power flow through transmission line $(i,j)\in\mathcal{L}$\\
   $\Tilde{P}_{i,j}$ && The post-islanding power flow through transmission line $(i,j)\in\mathcal{L}$\\
   $v_{i,k}$ && A binary indicator representing if reference generator $i=n_k$ belongs\\
   && to subsystem $\mathcal{G}_k$ ($v_{i,k}=1$) or not ($v_{i,k}=0$)\\
   $P_{d,i}$  && The power drawn from substation $i$ by load $d$\\
   $\underline{P}_{n,i}$ && The minimum power generation capacity of generator $n$\\
   $\Bar{P}_{n,i}$ && The maximum power generation capacity of generator $n$\\
   $\underline{\theta}_i$ && The minimum voltage angle of substation $i$\\
   $\Bar{\theta}_i$ && The maximum voltage angle of substation $i$\\
   $S_{i,j}$ && The susceptance of transmission line $(i,j)\in\mathcal{L}$
\end{tabular}

\subsection*{Variables}
\begin{tabular}{lll}
   $\mu$  &    &The islanding strategy of the grid operator\\
   $\pi$ && The power generation strategy of the grid operator\\
   $\tau $   && The transmission line removal strategy of the adversary\\
   $\gamma$ && The substation compromise strategy of the adversary\\
   $z_{i,j}^o$ && A binary variable indicating if transmission line $(i,j)\in\mathcal{L}$ is tripped\\
   && ($z_{i,j}^o=0$) or not ($z_{i,j}^o=1$) by the grid operator\\
   $z_{i,j}^a$ && A binary variable indicating if transmission line $(i,j)\in\mathcal{L}$ is tripped\\ &&($z_{i,j}^a=0$) or not ($z_{i,j}^a=1$) by the grid operator\\
   $r$ && The adversary's utility, i.e., the amount of power flow disruption that the\\
   && system incurs when the grid operator and adversary execute their\\
   &&equilibrium strategies\\
   $u_{z^oz^a}$ && An auxiliary variable defined as $u_{z^oz^a}=\mu(z^o)\tau(z^a)$\\
   $w_{i,j,k}$ && A binary variable indicating if transmission line $(i,j)$ belongs to\\
   &&subsystem $\mathcal{L}_k$ ($w_{i,j,k}=1$) or not ($w_{i,j,k}=0$)\\
   $x_{i,k}$ && A variable indicating if substation $i$ belongs to subsystem $\mathcal{G}_k$ ($x_{i,k}=1$)\\
   && or not ($x_{i,k}=0$)\\
   $f_{i,j,k}$ && A continuous variable that models a network flow in the power system\\
   $g_{n,i}$ && The power injected to substation $i$ from generator $n$\\
   $\theta_i$ && The voltage angle of substation $i$\\
   $y_i$ && A binary variable indicating if substation $i$ is compromised ($y_i=1$) or\\
   && not ($y_i=0$) by the adversary
\end{tabular}
